# Supplementary material for: Multi-objective Electric Vehicle Charging Strategies at Energy Hubs with Justice-informed Profit Distribution among Users
Source: arXiv:2611.08629 source file (2026-11-05)
Supplement: Supplementary file 1 [file Appendix_Nash.tex]

\subsection{2 step Nash}
Instead of a single optimisation we now first take an unweighted Nash equilibrium between the users and the station. Only then we divide this money between all users
% \begin{equation}
%     min ~(\varphi_{\mathrm{op}}) \cdot \left(\sum_{n=1}^{N_\mathrm{ev}}\varphi_{\mathrm{ev},n}\right) ~\text{ s.t. }~ \varphi_{\mathrm{op}}+\sum_{n=1}^{N_\mathrm{ev}}\varphi_{\mathrm{ev},n} = \varPhi
% \end{equation}
\begin{multline}
    \widetilde{J} = -\left(-\sum_{n=1}^{N_\mathrm{ev}}\varphi_{\mathrm{ev},n} + \varPhi + C_\mathrm{BESS}^\mathrm{nom} - C_\mathrm{BESS}\right) \\ \cdot \left(\sum_{n=1}^{N_\mathrm{ev}}\varphi_{\mathrm{ev},n} + C_\mathrm{evb}^\mathrm{nom} - C_\mathrm{evb} \right)% \\ ~\text{ s.t. }~ \varphi_{\mathrm{op}}+\sum_{n=1}^{N_\mathrm{ev}}\varphi_{\mathrm{ev},n} = \varPhi
\end{multline}
where we set $\sum_{n=1}^{N_\mathrm{ev}}\varphi_{\mathrm{ev},n} = \varPhi_{\mathrm{ev}}$ which is the total amount of money allocated to the EVs. Taking the log of each of the terms we get
\begin{multline}
    \widetilde{J} = -\log\left(-\varPhi_{\mathrm{ev}} + \varPhi + C_\mathrm{BESS}^\mathrm{nom} - C_\mathrm{BESS}\right) \\ - \log\left(\varPhi_{\mathrm{ev}} + C_\mathrm{evb}^\mathrm{nom} - C_\mathrm{evb} \right)
\end{multline}
\begin{equation}
    \min_{\varPhi_{\mathrm{ev}}}~\widetilde{J}
\end{equation}
This is an unconstrained problem, we take the partial derivative of $\widetilde{J}$ to $\varPhi_\mathrm{ev}$ and set it equal to $0$ to find the optimum
\begin{multline}
    \frac{1}{-\varPhi_{\mathrm{ev}} + \varPhi + C_\mathrm{BESS}^\mathrm{nom} - C_\mathrm{BESS}} \\ -\frac{1}{\varPhi_{\mathrm{ev}} + C_\mathrm{evb}^\mathrm{nom} - C_\mathrm{evb}} = 0
\end{multline}
\begin{multline}
    -\varPhi_{\mathrm{ev}} + \varPhi + C_\mathrm{BESS}^\mathrm{nom} - C_\mathrm{BESS} \\ = \varPhi_{\mathrm{ev}} + C_\mathrm{evb}^\mathrm{nom} - C_\mathrm{evb}
\end{multline}
working this out we get:
\begin{multline}
    \varPhi_{\mathrm{ev}} = 0.5\cdot\left(\varPhi + C_\mathrm{BESS}^\mathrm{nom} - C_\mathrm{BESS} - C_\mathrm{evb}^\mathrm{nom} + C_\mathrm{evb} \right)
\end{multline}
This means that the EVs get half of the profits, they pay for half of the amortisation increase of the BESS and get paid for half of the total EV battery amortisation increase.

\subsubsection*{Dividing among EVs}
Taking the money allocated to the EVs found in the previous section we take a weighted Nash equilibrium to find the allocation for each EV. 

% \begin{equation}
%     J = \prod_{n=1}^{N_\mathrm{ev}}\left(u_{\mathrm{ev}, n} - u_{\mathrm{ev}, n}^\mathrm{nom}\right)
% \end{equation}
\begin{equation}
    J = -\prod_{n=1}^{N_\mathrm{ev}}\left( \varphi_{\mathrm{ev}, n} + C_{\mathrm{evb}, n}^\mathrm{nom} - C_{\mathrm{evb}, n}\right)^{E_{\mathrm{ch}, n}}
\end{equation}
\begin{equation}
    J = -\sum_{n=1}^{N_\mathrm{ev}} E_{\mathrm{ch}, n} \cdot \log\left( \varphi_{\mathrm{ev}, n} + C_{\mathrm{evb}, n}^\mathrm{nom} - C_{\mathrm{evb}, n}\right)
\end{equation}
\begin{equation}
    \min_{\varphi} J ~\text{ s.t. }~ \sum_{n=1}^{N_\mathrm{ev}}\varphi_{\mathrm{ev}, n} = \varPhi_\mathrm{ev}
\end{equation}
We dualise this problem
\begin{multline}
    L(\varPhi_\mathrm{ev}, \lambda) = -\sum_{n=1}^{N_\mathrm{ev}} E_{\mathrm{ch}, n} \cdot \log\left( \varphi_{\mathrm{ev}, n} + C_{\mathrm{evb}, n}^\mathrm{nom} - C_{\mathrm{evb}, n}\right) \\ + \lambda\cdot\left(\sum_{n=1}^{N_\mathrm{ev}}\varphi_{\mathrm{ev}, n} - \varPhi_\mathrm{ev}\right)
\end{multline}

We take the derivative to find the optimum
\begin{equation}
    \frac{\partial L}{\partial \varphi_{\mathrm{ev}, n}} = \lambda - \frac{E_{\mathrm{ch}, n}}{\varphi_{\mathrm{ev}, n}^\star + C_{\mathrm{evb}, n}^\mathrm{nom} - C_{\mathrm{evb}, n}} = 0
\end{equation}
% \begin{equation}
%     \lambda = \frac{E_{\mathrm{ch}, n}}{\varphi_{\mathrm{ev}, n}^\star + C_{\mathrm{evb}, n}^\mathrm{nom} - C_{\mathrm{evb}, n}}
% \end{equation}
\begin{equation}
    \varphi_{\mathrm{ev}, n}^\star = \frac{E_{\mathrm{ch}, n}}{\lambda} - C_{\mathrm{evb}, n}^\mathrm{nom} + C_{\mathrm{evb}, n}
\end{equation}

Filling this in in the constraint gives
\begin{equation}
    \sum_{n=1}^{N_\mathrm{ev}} \frac{E_{\mathrm{ch}, n}}{\lambda} + \Delta C_{\mathrm{evb}, n} = \varPhi_\mathrm{ev}
\end{equation}
\begin{multline}
    \sum_{n=1}^{N_\mathrm{ev}} \frac{E_{\mathrm{ch}, n}}{\lambda} + \Delta C_{\mathrm{evb}, n} = \\ 0.5\cdot\left(\varPhi + \sum_{n=1}^{N_\mathrm{ev}} - \Delta C_{\mathrm{BESS}, n} + \Delta C_{\mathrm{evb}, n} \right)
\end{multline}
\begin{multline}
    \sum_{n=1}^{N_\mathrm{ev}} \frac{E_{\mathrm{ch}, n}}{\lambda} = \\ 0.5\cdot\left(\varPhi + \sum_{n=1}^{N_\mathrm{ev}} - \Delta C_{\mathrm{BESS}, n} - \Delta C_{\mathrm{evb}, n} \right)
\end{multline}
\begin{equation}
    \lambda = \frac{2\cdot\sum_{n=1}^{N_\mathrm{ev}} E_{\mathrm{ch}, n}}{\varPhi + \sum_{n=1}^{N_\mathrm{ev}} - \Delta C_{\mathrm{BESS}, n} - \Delta C_{\mathrm{evb}, n}}
\end{equation}
filling this back in gives:
\begin{equation}
    \varphi_{\mathrm{ev}, n}^\star = \frac{E_{\mathrm{ch}, n}\cdot\left(\varPhi + \sum_{n=1}^{N_\mathrm{ev}} - \Delta C_{\mathrm{BESS}, n} - \Delta C_{\mathrm{evb}, n}\right)}{2\cdot\sum_{n=1}^{N_\mathrm{ev}} E_{\mathrm{ch}, n}} + \Delta C_{\mathrm{evb}, n}
\end{equation}












\subsection{Nash equivalent to proportional allocation}

The weighted Nash welfare equation is 
% \begin{multline}
%     J = -F_\mathrm{op}(\varphi_{\mathrm{op}}) \cdot \prod_{n=1}^{N_\mathrm{ev}} F_n(\varphi_{\mathrm{ev}, n})^{E_{\mathrm{ch}, n}} \\ 
%     = -\log\left(F_\mathrm{op}(\varphi_{\mathrm{op}})\right)-\sum_{n=1}^{N_\mathrm{ev}}E_{\mathrm{ch}, n}\cdot \log\left(F_n(\varphi_{\mathrm{ev}, n})\right)
% \end{multline}
\begin{equation}
    J = -\prod_{n=1}^{N} F_n(\varphi_n)^{w_n} = -\sum_{n=1}^{N}w_n \cdot \log\left(F_n(\varphi_n)\right)
\end{equation}
where $\varphi_n$ is the amount of money allocated to agent $n$, $\varphi_n = C_{\mathrm{ev}, n}^\mathrm{nom} - C_{\mathrm{ev}, n}$, $F_n(\varphi)$ is each agent's cost profile, which depends on the total amount of money allocated to this agent and $w_n$ is the weight of each agent. This equation is the generalised form of~\cref{eq:NBS1}.

Assuming the charging scheduling problem and profit allocation problems are independent the profit allocation problem becomes
% \begin{equation}
%     \min_{\varphi_\star} J ~\text{ s.t. }~ \varphi_\mathrm{op} + \sum_{n=1}^{N_\mathrm{ev}}\varphi_{\mathrm{ev}, n} = \varPhi
% \end{equation}
\begin{equation}
    \min_{\varphi} ~ J(\mathbf{F}(\varphi)) ~\text{ s.t. }~ \sum_{n=1}^{N}\varphi_n = \varPhi
\end{equation}
where $\varPhi$ is the total profit generated through smart charging ($C_\mathrm{el}^\mathrm{nom} - C_\mathrm{el}$). % this is maximised in Problem~\ref{prob:simple_optimisation}

We dualise this problem, the corresponding Lagrangian is
\begin{equation}
    L(\varphi_n, \lambda) = -\sum_{n=1}^{N}w_n \cdot \log\left(F_n(\varphi_n)\right) + \lambda \cdot \left( \sum_{n=1}^{N}\varphi_n - \varPhi \right)
\end{equation}
where $\lambda$ is the dual variable of the constraint.

By principle of optimality we have
\begin{equation}
    \frac{\partial L}{\partial \varphi_n} = \lambda - \frac{w_n}{F_n(\varphi_n)} \cdot \frac{\partial F_n(\varphi_n)}{\partial \varphi_n} = 0
\end{equation}
assuming the functions $F_n$ are affine: $F_n(\varphi_n) = a_n\cdot\varphi_n+b_n$ we get
\begin{equation}
    \lambda = \frac{w_n}{\varphi_n^\star + b_n / a_n}
\end{equation}
\begin{equation}
    \varphi_n^\star = \frac{w_n}{\lambda}-\frac{b_n}{a_n},
\end{equation}
using primal feasibility yields
\begin{equation}
    \sum_{n=1}^{N} \frac{w_n}{\lambda} - \frac{b_n}{a_n} = \varPhi
\end{equation}
\begin{equation}
    \frac{\sum_{n=1}^{N} w_n}{\lambda} - \sum_{n=1}^{N} \frac{b_n}{a_n} = \varPhi
\end{equation}
\begin{equation}
    \frac{\sum_{n=1}^{N} w_n}{\varPhi + \sum_{n=1}^{N} \frac{b_n}{a_n}} = \lambda
\end{equation}

substituting this back we get
\begin{equation}
    \varphi_n^\star = \frac{w_n}{\sum_{n=1}^{N} w_n}\cdot\left(\varPhi + \sum_{n=1}^{N} \frac{b_n}{a_n}\right) - \frac{b_n}{a_n},
\end{equation}

For the case considered in appendix A of~\cite{ShilovElokdaEtAl2026} $b_n = 0$ we get
\begin{equation}
    \varphi_n^\star = \frac{w_n}{\sum_{n=1}^{N} w_n}\cdot\varPhi,
\end{equation}
which is the proportional allocation, as was found in~\cite{ShilovElokdaEtAl2026} as well.

In the problem described in \autoref{ch:Nash_theory} we have that $a_n = 1$ and $b_n = C_{\mathrm{evb}, n}^\mathrm{nom} - C_{\mathrm{evb}, n}$ is the change in battery amortisation costs. This results in the profits minus the sum of battery amortisation costs being proportionally split among users where each user is subsequently compensated for their increased battery amortisation. Which is what we observe.

Conclusion: OLC and Nash are nearly the same (in simple cases)
